# Supplementary material for: Third harmonic-mediated amplification in TWPA
Source: arXiv:2508.05295 source file (2025-11-03)
Supplement: Supplementary file 1 [file SI.pdf]

# Supplementary Material for "Third harmonic-mediated amplification in TWPA"

E. Rizvanov, S. Kern, P. Neilinger, and M. Grajcar

Department of Experimental Physics, Comenius University, SK-84248 Bratislava, Slovakia

In the supplementary material, we derived the dispersion relation for a single unit cell of PTWPA, obtained the sweet spot analytically, provided the full set of equations of CMT-3 and the simplified CMT, and compared JoSIM and WRspice.

## S1. JOSIM AND WRSPICE COMPARISON

At the optimal working point the power flow for main harmonics in JoSIM and WRspice are approximately the same (Fig. 1). For the details of simulations settings see Ref.1.

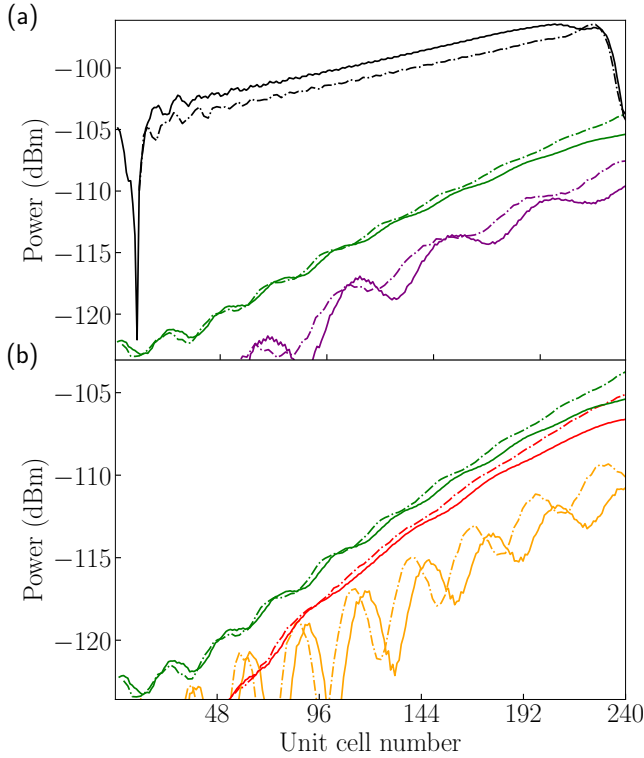

FIG. 1. Power flow of propagating plane waves for relevant modes simulated in JoSIM (solid line) and WRspice (dash-dotted line) for  $I_s = 0.01 \mu\text{A}$ ,  $I_{dc} = 0.8 \mu\text{A}$ ,  $f_p = 8.64 \text{ GHz}$  and  $f_s = 4.8 \text{ GHz}$  (purple). Pump amplitudes are different in JoSIM ( $I_p = 1.6 \mu\text{A}$ ) and WRspice ( $I_p = 1.65 \mu\text{A}$ ). a)  $f_{3p}$  (black line),  $f_s$  (green line),  $f_{p+s}$  (purple line); b)  $f_s$  (green line),  $f_{2p-s}$  (red line),  $f_{p-s}$  (orange line).

## S2. DISPERSION RELATION

The ABCD matrix of a single junction in a Unit Cell in Fig.1 (b) is:

$$M_{JJ} = \begin{pmatrix} 1 - \frac{\omega^2 LC_g}{i\omega C_g} & \frac{i\omega L}{1 - \omega^2 LC_{JJ}} \\ \frac{i\omega L}{1 - \omega^2 LC_{JJ}} & 1 \end{pmatrix}, \quad (\text{S1})$$

and the ABCD matrix of a junction with additional capacitance is:

$$M_p = \begin{pmatrix} 1 - \frac{\omega^2 LC_g}{1 - \omega^2 L(C_{JJ} + C_p)} & \frac{i\omega L}{1 - \omega^2 L(C_{JJ} + C_p)} \\ \frac{i\omega C_g}{1} & 1 \end{pmatrix}, \quad (\text{S2})$$

where the junction inductance is:

$$L = \frac{\Phi_0}{(2\pi I_c)} (1 + I_d^2 / (2I_c^2)). \quad (\text{S3})$$

The matrix of the unit cell is then given:

$$M = \begin{pmatrix} A & B \\ C & D \end{pmatrix} = M_{JJ}^{-1} \cdot M_p. \quad (\text{S4})$$

Using the matrix elements, we can approximate the wave vector<sup>2</sup>:

$$k \approx \frac{1}{ndz} \arccos \left( \frac{A + D}{2} \right) = \frac{1}{dx} \arccos \left( \frac{A + D}{2} \right). \quad (\text{S5})$$

This way, we estimated the wave vector from a single unit cell (see Fig.4 (a)).

## S3. THIRD HARMONIC GENERATION OF THE PUMP

To explain the nature of the sweet spot, i.e., a narrow band for the pump frequency, where the gain was observed, and to support the assumption regarding the impact of the third harmonic on the transmission (see Fig.1 (c)), we first analyze the case involving only two waves; the pump and its third harmonic:

$$I = \frac{1}{2} I_p(x) \exp(i(k_p x - \omega_p t)) + \frac{1}{2} I_{3p}(x) \exp(i(k_{3p} x - 3\omega_p t)) + C.C.; \quad (\text{S6})$$

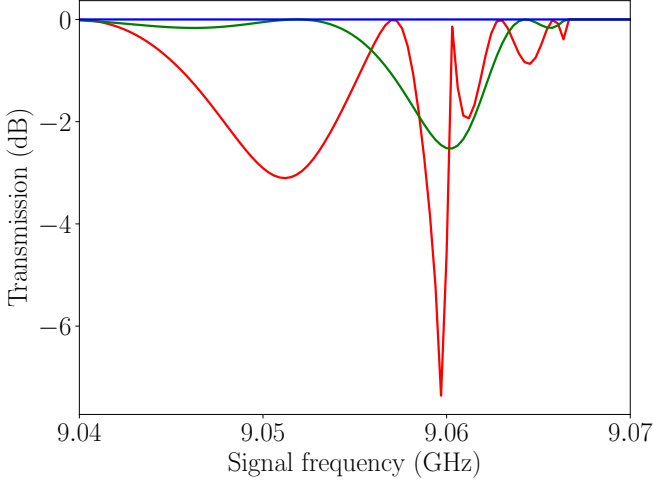

FIG. 2. PTWPA Transmission spectra ( $S_{21}$ ) of single pump tone given by Eq.(S7) and Eq.(S8) for different powers. Parameters of the simulation are:  $I_p = 1$  uA (red line),  $I_p = 0.5$  uA (green line),  $I_p = 0.01$  uA (blue line),  $I_d = 0.8$  uA.

Plugging this anzatz to Eq. 1, we obtain:

$$\frac{dI_p}{dx} = i \frac{k_p \xi}{24} (6 |I_{3p}|^2 I_p + 3 |I_p|^2 + 3 I_{3p} e^{ix(k_{3p} - 3k_p)} (I_p^*)^2), \quad (\text{S7})$$

$$\frac{dI_{3p}}{dx} = i \frac{k_{3p} \xi}{24} (3 I_{3p} |I_{3p}|^2 + 3 I_{3p} |I_p|^2 + I_p^3 e^{ix(-k_{3p} + 3k_p)}). \quad (\text{S8})$$

The dispersion (Fig. 4 (a)) and the transmission (Fig.1 (c)) allow us to set  $k_{3p}$  to be in the stopband ( $\text{Im}(k_{3p}) \neq 0$ ), where we assume  $I_{3p} = 0$ . Solving this system of equations, we obtain a similar sweet spot (Fig.2) as was obtained in JoSIM simulations (Fig.1 (d)). The sweet spot in this case is noticeably narrower than in simulations (Fig.1 (d)). This may be caused by the approximate dispersion relation (see Section S2).

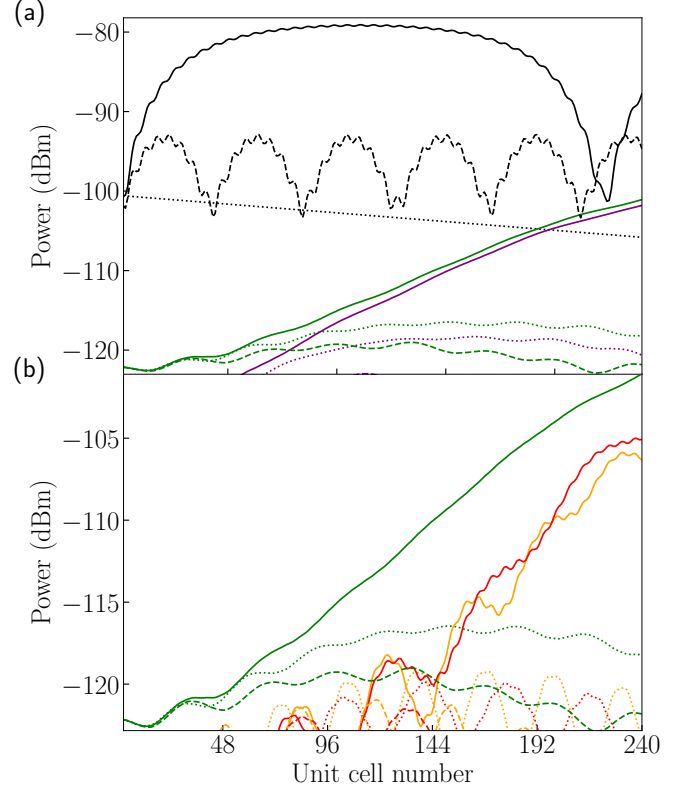

FIG. 3. Power flow for relevant modes according to CMT-3. a)  $f_{3p}$  (black line),  $f_s$  (green line),  $f_{p+s}$  (purple line); b)  $f_s$  (green line),  $f_{2p-s}$  (red line),  $f_{p-s}$  (orange line). Calculation was done by Explicit Runge-Kutta method of order 3(2). Parameters of the simulation are:  $f_s = 4.8$  GHz;  $f_p = 8.912$  GHz (dashed line);  $f_p = 9.062$  GHz (solid line);  $f_p = 9.212$  GHz (dotted line),  $I_{p0} = 1$   $\mu$ A,  $I_{s0} = 0.005$   $\mu$ A,  $I_d = 0.8$   $\mu$ A. From Eq.S5:  $\Delta k_{3p} = 0.0008$  for  $f_p = 9.061$  GHz;  $\Delta k_{3p} = 0.0352$  for  $f_p = 8.911$  GHz;  $\Delta k_{3p} = 0.0017$  for  $f_p = 9.211$  GHz, where  $\Delta k_{3p} = k_{3p} - 3k_p$ . Initial conditions for whole set of harmonics:  $I_s(0) = I_{s0}$ ,  $I_p(0) = I_{p0}$ ,  $I_{2p}(0) = 0.08 I_p(0)$ ,  $I_{3p}(0) = 0.06 I_p(0)$ ;  $I_\alpha(0) = 0$ ,  $\alpha \in \{p-s, p+s, 2p-s, 2p+s, 3p-s\}$ .

#### S4. CMT-3

Motivated by our numerical simulations we included the second  $f_{2p}$  and the third harmonic  $f_{3p}$  of the pump, as well as pump-mediated sum-frequency tones:  $f_{p-s}$ ,  $f_{p+s}$ ,  $f_{2p-s}$ ,  $f_{2p+s}$ ,  $f_{3p-s}$ . We assumed the signal to be much weaker than the pump, neglecting the second and the higher-order sidebands as in Ref.<sup>3</sup>:

$$I = \sum_{\alpha} \frac{1}{2} I_{\alpha}(x) \exp(i(k_{\alpha}x - \omega_{\alpha}t)) + C.C, \quad (S9)$$

$$\alpha \in \{s, p-s, p, p+s, 2p-s, 2p, 2p+s, 3p-s, 3p\}.$$

If  $-k_{3p} + 3k_p = \Delta k_{3p} = 0$ , the leading term for THG in Eq.S12 is:

$$i \frac{k_{3p}\xi}{24} I_p^3 e^{ix(-k_{3p}+3k_p)}, \quad (S10)$$

since  $I_p$  is much higher than other harmonics and will be dominant.

Figure 3 (a) shows that the qualitative behavior predicted by the extended CMT is consistent with the simulation results. In particular, smaller values of  $\Delta k_{3p}$  lead to higher gain and a significant increase in the third harmonic amplitude. This is strongly correlated with enhanced signal gain as illustrated by the comparison of solid, dashed, and dotted green lines in Fig. 3 (a). Moreover, the result for sideband  $f_{p+s}$ , which increases along the signal in the case of the matched third harmonic (see Fig. 3 (a)), supports the analysis presented in the previous section.

The discrepancy between the theory and the simulations may be caused by a restricted number of harmonics considered in the theory<sup>4,5</sup> as well as by neglecting the reflections<sup>6,7</sup>, and the power dependence of the dispersion itself<sup>8</sup>.

The second and third harmonic of the pump can be in the stopband and have an imaginary part in  $k_{2p,3p}$  (see Fig.4 (a)), which leads to divergencies in the CMT<sup>4,5</sup>. The imaginary part of the k-vector corresponds to attenuation<sup>2</sup>. We used a simple approximation directly including attenuation to the equation for second harmonics in a similar way as was done in Ref.<sup>9</sup>:

$$\frac{dI_{2p,3p}}{dx} = -\delta_{2p,3p} \text{Im}(k_{2p,3p}) I_{2p,3p}, \quad (S11)$$

where  $\delta_{2p,3p}$  is the attenuation constant which we estimated from numerical simulations (see Fig.2). In our case, we set  $\delta_{2p} = 0.00032$ ,  $\delta_{3p} = 0.01$ . Substituting ansatz Eq.S9 to Eq.1, the following set of equations is obtained:

$$\begin{aligned} \frac{dI_{3p}}{dx} = & i \frac{k_{3p}\epsilon}{8} \left[ 2I_{3p-s}I_s e^{ix(k_{3p-s}-k_{3p}+k_s)} + 2I_{2p}I_p e^{ix(k_{2p}-k_{3p}+k_p)} + 2I_{2p+s}I_{p-s} e^{ix(k_{2p+s}-k_{3p}+k_{p-s})} \right. \\ & \left. + 2I_{2p-s}I_{p+s} e^{ix(-k_{3p}+k_{2p-s}+k_{p+s})} \right] \\ & + i \frac{k_{3p}\xi}{24} \left( 6I_{3p-s}I_{2p} e^{ix(k_{3p-s}+k_{2p}-k_{3p}-k_{2p-s})} I_{2p-s}^* + 6I_{3p-s}I_{2p+s} e^{ix(k_{3p-s}-k_{2p}+k_{2p+s}-k_{3p})} I_{2p}^* \right. \\ & + 6I_{3p-s}I_{3p}I_{3p-s}^* + 6iI_{3p-s}I_p k_{3p}\xi e^{ix(k_{3p-s}-k_{3p}-k_{p-s}+k_p)} I_{p-s}^* \\ & + 6I_{3p-s}I_{p+s} e^{ix(k_{3p-s}-k_{3p}-k_p+k_{p+s})} I_p^* + 3I_{2p}^2 e^{ix(2k_{2p}-k_{3p}-k_p)} I_p^* \\ & + 6I_{2p}I_{2p+s} e^{ix(k_{2p}+k_{2p+s}-k_{3p}-k_{p+s})} I_{p+s}^* + 6I_{2p}I_{3p}I_{2p}^* \\ & + 6I_{2p}I_{p-s}I_s e^{ix(k_{2p}-k_{3p}+k_{p-s}+k_s)} + 6I_{2p}I_{2p-s} e^{ix(k_{2p}-k_{3p}-k_{p-s}+k_{2p-s})} I_{p-s}^* \\ & + 6I_{2p}I_{p+s} e^{ix(k_{2p}-k_{3p}+k_{p+s}-k_s)} I_s^* + 6I_{2p+s}I_{3p}I_{2p+s}^* \\ & + 6I_{2p+s}I_{2p-s} e^{ix(k_{2p+s}-k_{3p}+k_{2p-s}-k_p)} I_p^* + 6I_{2p+s}I_p e^{ix(k_{2p+s}-k_{3p}+k_p-k_s)} I_s^* \\ & + 3I_{3p}^2 I_{3p}^* + 6I_{3p}I_{p-s}I_{p-s}^* + 6I_{3p}I_{2p-s}I_{2p-s}^* + 6I_{3p}I_p I_p^* + 6I_{3p}I_{p+s}I_{p+s}^* \\ & + 6I_{3p}I_s I_s^* + 6I_{p-s}I_p I_{p+s} e^{ix(-k_{3p}+k_{p-s}+k_p+k_{p+s})} + 6I_{2p-s}I_p I_s e^{ix(-k_{3p}+k_{2p-s}+k_p+k_s)} \\ & \left. + I_p^3 e^{ix(-k_{3p}+3k_p)} \right) \end{aligned} \quad (S12)$$

$$\begin{aligned}
\frac{dI_{3p-s}}{dx} = & i \frac{k_{3p-s}\epsilon}{8} \left[ I_{2p} I_i e^{ix(-k_{3p-s}+k_{2p}+k_i)} + I_{3p} e^{ix(-k_{3p-s}+k_{3p}-k_s)} I_s^* + I_{ip} I_p e^{ix(-k_{3p-s}+k_{ip}+k_p)} \right] \\
& + i \frac{k_{3p-s}\xi}{24} \left( 3I_{3p-s}^2 I_{3p-s}^* + 6I_{3p-s} I_{2p} I_{2p}^* + 6I_{3p-s} I_{2p+s} I_{2p+s}^* + 6I_{3p-s} I_{3p} I_{3p}^* \right. \\
& + 6I_{3p-s} I_{p-s} I_{p-s}^* + 6I_{3p-s} I_{2p-s} I_{2p-s}^* + 6I_{3p-s} I_p I_p^* + 6I_{3p-s} I_{p+s} I_{p+s}^* \\
& + 6I_{3p-s} I_s I_s^* + 3I_{2p}^2 e^{ix(-k_{3p-s}+2k_{2p}-k_{p+s})} I_{p+s}^* + 6I_{2p} I_{3p} e^{ix(-k_{3p-s}+k_{2p}-k_{2p+s}+k_{3p})} I_{2p+s}^* \\
& + 6I_{2p} I_{2p-s} e^{ix(-k_{3p-s}+k_{2p}+k_{2p-s}-k_p)} I_p^* + 6I_{2p} I_p e^{ix(-k_{3p-s}+k_{2p}+k_p-k_s)} I_s^* \\
& + 6I_{2p+s} I_{p-s} e^{ix(-k_{3p-s}+k_{2p+s}+k_{p-s}-k_s)} I_s^* + 6I_{2p+s} I_{2p-s} e^{ix(-k_{3p-s}+k_{2p+s}+k_{2p-s}-k_{p+s})} I_{p+s}^* \\
& + 6I_{3p} I_{p-s} e^{ix(-k_{3p-s}+k_{3p}+k_{p-s}-k_p)} I_p^* + 6I_{3p} I_{2p-s} e^{ix(-k_{3p-s}-k_{2p}+k_{3p}+k_{2p-s})} I_{2p}^* \\
& + 6I_{3p} I_p e^{ix(-k_{3p-s}+k_{3p}+k_p-k_{p+s})} I_{p+s}^* + 3I_{p-s}^2 I_{p+s} e^{ix(-k_{3p-s}+2k_{p-s}+k_{p+s})} \\
& + 6I_{p-s} I_{2p-s} I_s e^{ix(-k_{3p-s}+k_{p-s}+k_{2p-s}+k_s)} + 3I_{p-s} I_p^2 e^{ix(-k_{3p-s}+k_{p-s}+2k_p)} \\
& \left. + 3I_{2p-s}^2 e^{ix(-k_{3p-s}-k_{p-s}+2k_{2p-s})} I_{p-s}^* + 6I_{2p-s} I_{p+s} e^{ix(-k_{3p-s}+k_{2p-s}+k_{p+s}-k_s)} I_s^* \right) \quad (S13)
\end{aligned}$$

$$\begin{aligned}
\frac{dI_{2p+s}}{dx} = & i \frac{k_{2p+s}\epsilon}{8} \left[ 2I_{2p} I_s e^{ix(k_{2p}-k_{2p+s}+k_s)} + 2I_{3p} e^{ix(-k_{2p+s}+k_{3p}-k_{p-s})} I_{p-s}^* + 2I_p I_{p+s} e^{ix(-k_{2p+s}+k_p+k_{p+s})} \right] \\
& + i \frac{k_{2p+s}\xi}{24} \left( 6I_{3p-s} I_{2p+s} I_{3p-s}^* + 6I_{3p-s} I_{p+s} e^{ix(k_{3p-s}-k_{2p+s}-k_{2p-s}+k_{p+s})} I_{2p-s}^* \right. \\
& + 6I_{3p-s} I_s e^{ix(k_{3p-s}-k_{2p+s}-k_{p-s}+k_s)} I_{p-s}^* + 3I_{2p}^2 e^{ix(2k_{2p}-k_{2p+s}-k_{2p-s})} I_{2p-s}^* \\
& + 6I_{2p} I_{2p+s} I_{2p}^* + 6I_{2p} I_{3p} e^{ix(-k_{3p-s}+k_{2p}-k_{2p+s}+k_{3p})} I_{3p-s}^* \\
& + 6I_{2p} I_p e^{ix(k_{2p}-k_{2p+s}-k_{p-s}+k_p)} I_{p-s}^* + 6I_{2p} I_{p+s} e^{ix(k_{2p}-k_{2p+s}-k_p+k_{p+s})} I_p^* \\
& + 3I_{2p+s}^2 I_{2p+s}^* + 6I_{2p+s} I_{3p} I_{3p}^* + 6I_{2p+s} I_{p-s} I_{p-s}^* + 6I_{2p+s} I_{2p-s} I_{2p-s}^* \\
& + 6I_{2p+s} I_p I_p^* + 6I_{2p+s} I_{p+s} I_{p+s}^* + 6I_{2p+s} I_s I_s^* + 6I_{3p} I_p e^{ix(-k_{2p+s}+k_{3p}-k_{2p-s}+k_p)} I_{2p-s}^* \\
& + 6I_{3p} I_{p+s} e^{ix(-k_{2p}-k_{2p+s}+k_{3p}+k_{p+s})} I_{2p}^* + 6I_{3p} I_s e^{ix(-k_{2p+s}+k_{3p}-k_p+k_s)} I_p^* \\
& + 6I_{p-s} I_{p+s} I_s e^{ix(-k_{2p+s}+k_{p-s}+k_{p+s}+k_s)} + 6I_{2p-s} I_{p+s} e^{ix(-k_{2p+s}-k_{p-s}+k_{2p-s}+k_{p+s})} I_{p-s}^* \\
& \left. + 3I_{2p-s} I_s^2 e^{ix(-k_{2p+s}+k_{2p-s}+2k_s)} + 3I_p^2 I_s e^{ix(-k_{2p+s}+2k_p+k_s)} + 3I_{p+s}^2 e^{ix(-k_{2p+s}+2k_{p+s}-k_s)} I_s^* \right) \quad (S14)
\end{aligned}$$

$$\begin{aligned}
\frac{dI_{2p}}{dx} = & i \frac{k_{2p}\epsilon}{8} \left[ I_{3p-s} e^{ix(k_{3p-s}-k_{2p}-k_{p-s})} I_i^* + I_{2p+s} e^{ix(-k_{2p}+k_{2p+s}-k_s)} I_s^* + I_{3p} e^{ix(-k_{2p}+k_{3p}-k_p)} I_p^* \right. \\
& \left. + I_{p-s} I_{p+s} e^{ix(-k_{2p}+k_{p-s}+k_{p+s})} + I_{2p-s} I_s e^{ix(-k_{2p}+k_{2p-s}+k_s)} + I_p^2 e^{ix(-k_{2p}+2k_p)} \right] \\
& + i \frac{k_{2p}\xi}{24} \left( I_{3p-s} I_{2p} I_{3p-s}^* + I_{3p-s} I_{2p+s} e^{ix(k_{3p-s}-k_{2p}+k_{2p+s}-k_{3p})} I_{3p}^* \right. \\
& + I_{3p-s} I_p e^{ix(k_{3p-s}-k_{2p}-k_{2p-s}+k_p)} I_{2p-s}^* + I_{3p-s} I_{p+s} e^{ix(k_{3p-s}-2k_{2p}+k_{p+s})} I_{2p}^* \\
& + I_{3p-s} I_s e^{ix(k_{3p-s}-k_{2p}-k_p+k_s)} I_p^* + I_{2p}^2 I_{2p}^* + I_{2p} I_{2p+s} I_{2p+s}^* + I_{2p} I_{3p} I_{3p}^* \\
& + I_{2p} I_{p-s} I_{p-s}^* + I_{2p} I_{2p-s} I_{2p-s}^* + I_{2p} I_p I_p^* + I_{2p} I_{p+s} I_{p+s}^* + I_{2p} I_s I_s^* \\
& + I_{2p+s} I_{p-s} e^{ix(-k_{2p}+k_{2p+s}+k_{p-s}-k_p)} I_p^* + I_{2p+s} I_{2p-s} e^{ix(-2k_{2p}+k_{2p+s}+k_{2p-s})} I_{2p}^* \\
& + I_{2p+s} I_p e^{ix(-k_{2p}+k_{2p+s}+k_p-k_{p+s})} I_{p+s}^* + I_{3p} I_{p-s} e^{ix(-k_{2p}+k_{3p}+k_{p-s}-k_{2p-s})} I_{2p-s}^* \\
& + I_{3p} I_{2p-s} e^{ix(-k_{3p-s}-k_{2p}+k_{3p}+k_{2p-s})} I_{3p-s}^* + I_{3p} I_p e^{ix(-2k_{2p}+k_{3p}+k_p)} I_{2p}^* \\
& + I_{3p} I_{p+s} e^{ix(-k_{2p}-k_{2p+s}+k_{3p}+k_{p+s})} I_{2p+s}^* + I_{3p} I_s e^{ix(-k_{2p}+k_{3p}-k_{p+s}+k_s)} I_{p+s}^* \\
& + I_{3p} e^{ix(-k_{2p}+k_{3p}-k_{p-s}-k_s)} I_i^* I_s^* + I_{p-s} I_p I_s e^{ix(-k_{2p}+k_{p-s}+k_p+k_s)} \\
& + I_{2p-s} I_p e^{ix(-k_{2p}-k_{p-s}+k_{2p-s}+k_p)} I_{p-s}^* + I_{2p-s} I_{p+s} e^{ix(-k_{2p}+k_{2p-s}-k_p+k_{p+s})} I_p^* \\
& \left. + I_p I_{p+s} e^{ix(-k_{2p}+k_p+k_{p+s}-k_s)} I_s^* \right) \tag{S15}
\end{aligned}$$

$$\begin{aligned}
\frac{dI_{2p-s}}{dx} = & i \frac{k_{2p-s}\epsilon}{8} \left[ 2I_{3p-s} e^{ix(k_{3p-s}-k_{2p-s}-k_p)} I_p^* + 2I_{2p} e^{ix(k_{2p}-k_{2p-s}-k_s)} I_s^* + 2I_{3p} e^{ix(k_{3p}-k_{2p-s}-k_{p+s})} I_{p+s}^* \right. \\
& \left. + 2I_{p-s} I_p e^{ix(k_{p-s}-k_{2p-s}+k_p)} \right] \\
& + i \frac{k_{2p-s}\xi}{24} \left( 6I_{3p-s} I_{2p} e^{ix(k_{3p-s}+k_{2p}-k_{3p}-k_{2p-s})} I_{3p}^* + 6I_{3p-s} I_{p-s} e^{ix(k_{3p-s}+k_{p-s}-2k_{2p-s})} I_{2p-s}^* \right. \\
& + 6I_{3p-s} I_{2p-s} I_{3p-s}^* + 6I_{3p-s} I_p e^{ix(k_{3p-s}-k_{2p}-k_{2p-s}+k_p)} I_{2p}^* \\
& + 6I_{3p-s} I_{p+s} e^{ix(k_{3p-s}-k_{2p+s}-k_{2p-s}+k_{p+s})} I_{2p+s}^* + 6I_{3p-s} I_s e^{ix(k_{3p-s}-k_{2p-s}-k_{p+s}+k_s)} I_{p+s}^* \\
& + 6I_{3p-s} e^{ix(k_{3p-s}-k_{p-s}-k_{2p-s}-k_s)} I_{p-s}^* I_s^* + 3I_{2p}^2 e^{ix(2k_{2p}-k_{2p+s}-k_{2p-s})} I_{2p+s}^* \\
& + 6I_{2p} I_{p-s} e^{ix(k_{2p}+k_{p-s}-k_{2p-s}-k_p)} I_p^* + 6I_{2p} I_{2p-s} I_{2p}^* + 6I_{2p} I_p e^{ix(k_{2p}-k_{2p-s}+k_p-k_{p+s})} I_{p+s}^* \\
& + 6I_{2p+s} I_{p-s} e^{ix(k_{2p+s}+k_{p-s}-k_{2p-s}-k_{p+s})} I_{p+s}^* + 6I_{2p+s} I_{2p-s} I_{2p+s}^* \\
& + 3i I_{2p+s} k_{2p-s} \xi e^{ix(k_{2p+s}-k_{2p-s}-2k_s)} (I_s^*)^2 + 6I_{3p} I_{p-s} e^{ix(-k_{2p}+k_{3p}+k_{p-s}-k_{2p-s})} I_{2p}^* \\
& + 6I_{3p} I_{2p-s} I_{3p}^* + 6I_{3p} I_p e^{ix(-k_{2p+s}+k_{3p}-k_{2p-s}+k_p)} I_{2p+s}^* \\
& + 6I_{3p} e^{ix(k_{3p}-k_{2p-s}-k_p-k_s)} I_p^* I_s^* + 3I_{p-s}^2 I_s e^{ix(2k_{p-s}-k_{2p-s}+k_s)} \\
& + 6I_{p-s} I_{2p-s} I_{p-s}^* + 6I_{p-s} I_{p+s} e^{ix(k_{p-s}-k_{2p-s}+k_{p+s}-k_s)} I_s^* + 3I_{2p-s}^2 I_{2p-s}^* + 6I_{2p-s} I_p I_p^* \\
& \left. + 6I_{2p-s} I_{p+s} I_{p+s}^* + 6I_{2p-s} I_s I_s^* + 3I_p^2 e^{ix(-k_{2p-s}+2k_p-k_s)} I_s^* \right) \tag{S16}
\end{aligned}$$

$$\begin{aligned}
\frac{dI_{p+s}}{dx} = & i \frac{k_{p+s}\epsilon}{8} \left[ 2I_{2p}e^{ix(k_{2p}-k_{p-s}-k_{p+s})}I_{p-s}^* + 2I_{2p+s}e^{ix(k_{2p+s}-k_p-k_{p+s})}I_p^* + 2I_{3p}e^{ix(k_{3p}-k_{2p-s}-k_{p+s})}I_{2p-s}^* \right. \\
& \left. + 2I_pI_s e^{ix(k_p-k_{p+s}+k_s)} \right] \\
& + i \frac{k_{p+s}\xi}{24} \left( 6I_{3p-s}I_s e^{ix(k_{3p-s}-k_{2p-s}-k_{p+s}+k_s)}I_{2p-s}^* + 3I_{3p-s}e^{ix(k_{3p-s}-2k_{p-s}-k_{p+s})}(I_{p-s}^*)^2 \right. \\
& + 3I_{2p}^2 e^{ix(-k_{3p-s}+2k_{2p}-k_{p+s})}I_{3p-s}^* + 6I_{2p}I_{2p+s}e^{ix(k_{2p}+k_{2p+s}-k_{3p}-k_{p+s})}I_{3p}^* \\
& + 6I_{2p}I_{p+s}I_{2p}^* + 6I_{2p}I_s e^{ix(k_{2p}-k_p-k_{p+s}+k_s)}I_p^* + 6I_{2p+s}I_{p-s}e^{ix(k_{2p+s}+k_{p-s}-k_{2p-s}-k_{p+s})}I_{2p-s}^* \\
& + 6I_{2p+s}I_{2p-s}e^{ix(-k_{3p-s}+k_{2p+s}+k_{2p-s}-k_{p+s})}I_{3p-s}^* + 6I_{2p+s}I_{p+s}I_{2p+s}^* + 6I_{2p+s}I_s e^{ix(k_{2p+s}-2k_{p+s}+k_s)}I_{p+s}^* \\
& + 6I_{2p+s}e^{ix(k_{2p+s}-k_{p-s}-k_{p+s}-k_s)}I_{p-s}^*I_s^* + 6I_{3p}I_p e^{ix(-k_{3p-s}+k_{3p}+k_p-k_{p+s})}I_{3p-s}^* + 6I_{3p}I_{p+s}I_{3p}^* \\
& + 6I_{3p}I_s e^{ix(-k_{2p}+k_{3p}-k_{p+s}+k_s)}I_{2p}^* + 6I_{3p}e^{ix(k_{3p}-k_{p-s}-k_p-k_{p+s})}I_{p-s}^*I_p^* + 6I_{p-s}I_{p+s}I_{p-s}^* \\
& + 3I_{p-s}I_s^2 e^{ix(k_{p-s}-k_{p+s}+2k_s)} + 6I_{2p-s}I_{p+s}I_{2p-s}^* + 6I_{2p-s}I_s e^{ix(-k_{p-s}+k_{2p-s}-k_{p+s}+k_s)}I_{p-s}^* \\
& + 3I_p^2 e^{ix(-k_{p-s}+2k_p-k_{p+s})}I_{p-s}^* + 6I_pI_{p+s}I_p^* + 3I_{p+s}^2 I_{p+s}^* + 6I_{p+s}I_s I_s^* + 6I_{3p-s}I_{p+s}I_{3p-s}^* \\
& \left. + 6I_{2p}I_p e^{ix(k_{2p}-k_{2p-s}+k_p-k_{p+s})}I_{2p-s}^* + 6I_{2p+s}I_p e^{ix(-k_{2p}+k_{2p+s}+k_p-k_{p+s})}I_{2p}^* \right)
\end{aligned} \tag{S17}$$

$$\begin{aligned}
\frac{dI_p}{dx} = & i \frac{k_p\epsilon}{8} \left[ 2I_{3p-s}e^{ix(k_{3p-s}-k_{2p-s}-k_p)}I_{2p-s}^* + 2I_{2p}e^{ix(k_{2p}-2k_p)}I_p^* + 2I_{2p+s}e^{ix(k_{2p+s}-k_p-k_{p+s})}I_{p+s}^* \right. \\
& + 2I_{3p}e^{ix(-k_{2p}+k_{3p}-k_p)}I_{2p}^* + 2I_{p-s}I_s e^{ix(k_{p-s}-k_p+k_s)} + 2I_{2p-s}e^{ix(-k_{p-s}+k_{2p-s}-k_p)}I_{p-s}^* \\
& \left. + 2I_{p+s}e^{ix(-k_p+k_{p+s}-k_s)}I_s^* \right] \\
& + i \frac{k_p\xi}{24} \left( 6I_{3p-s}I_pI_{3p-s}^* + 6I_{3p-s}I_{p+s}e^{ix(k_{3p-s}-k_{3p}-k_p+k_{p+s})}I_{3p}^* + 6I_{3p-s}I_s e^{ix(k_{3p-s}-k_{2p}-k_p+k_s)}I_{2p}^* \right. \\
& + 6I_{3p-s}e^{ix(k_{3p-s}-k_{p-s}-2k_p)}I_{p-s}^*I_p^* + 3I_{2p}^2 e^{ix(2k_{2p}-k_{3p}-k_p)}I_{3p}^* \\
& + 6I_{2p}I_{p-s}e^{ix(k_{2p}+k_{p-s}-k_{2p-s}-k_p)}I_{2p-s}^* + 6I_{2p}I_{2p-s}e^{ix(-k_{3p-s}+k_{2p}+k_{2p-s}-k_p)}I_{3p-s}^* + 6I_{2p}I_pI_{2p}^* \\
& + 6I_{2p}I_{p+s}e^{ix(k_{2p}-k_{2p+s}-k_p+k_{p+s})}I_{2p+s}^* + 6I_{2p}I_s e^{ix(k_{2p}-k_p-k_{p+s}+k_s)}I_{p+s}^* \\
& + 6I_{2p}e^{ix(k_{2p}-k_{p-s}-k_p-k_s)}I_{p-s}^*I_s^* + 6I_{2p+s}I_{p-s}e^{ix(-k_{2p}+k_{2p+s}+k_{p-s}-k_p)}I_{2p}^* \\
& + 6I_{2p+s}I_pI_{2p+s}^* + 6I_{2p+s}e^{ix(k_{2p+s}-2k_p-k_s)}I_{p-s}^*I_s^* \\
& + 6I_{3p}I_{p-s}e^{ix(-k_{3p-s}+k_{3p}+k_{p-s}-k_p)}I_{3p-s}^* + 6I_{3p}I_pI_{3p}^* + 6iI_{3p}I_s k_p \xi e^{ix(-k_{2p+s}+k_{3p}-k_p+k_s)}I_{2p+s}^* \\
& + 3I_{3p}e^{ix(k_{3p}-3k_p)}(I_p^*)^2 + 6I_{3p}e^{ix(k_{3p}-k_{p-s}-k_p-k_{p+s})}I_{p-s}^*I_{p+s}^* \\
& + 6I_{3p}e^{ix(k_{3p}-k_{2p-s}-k_p-k_s)}I_{2p-s}^*I_s^* + 6I_{p-s}I_pI_{p-s}^* + 6I_{p-s}I_{p+s}e^{ix(k_{p-s}-2k_p+k_{p+s})}I_p^* \\
& + 6I_{2p-s}I_pI_{2p-s}^* + 6I_{2p-s}I_{p+s}e^{ix(-k_{2p}+k_{2p-s}-k_p+k_{p+s})}I_{2p}^* + 6I_{2p-s}I_s e^{ix(k_{2p-s}-2k_p+k_s)}I_p^* \\
& \left. + 3I_p^2 I_p^* + 6I_pI_{p+s}I_{p+s}^* + 6I_pI_s I_s^* + 6I_{2p+s}I_{2p-s}e^{ix(k_{2p+s}-k_{3p}+k_{2p-s}-k_p)}I_{3p}^* \right)
\end{aligned} \tag{S18}$$

$$\begin{aligned}
\frac{dI_{p-s}}{dx} = & i \frac{k_{p-s}}{8} \left[ 2iI_{3p-s}\epsilon k_{p-s} e^{ix(k_{3p-s}-k_{2p}-k_{p-s})} I_{2p}^* + 2iI_{2p}\epsilon k_{p-s} e^{ix(k_{2p}-k_{p-s}-k_{p+s})} I_{p+s}^* \right. \\
& + 2iI_{3p}k_{p-s} e^{ix(-k_{2p+s}+k_{3p}-k_{p-s})} I_{2p+s}^* + 2iI_{2p-s}\epsilon k_{p-s} e^{ix(-k_{p-s}+k_{2p-s}-k_p)} I_p^* + 2iI_p\epsilon k_{p-s} e^{ix(-k_{p-s}+k_p-k_s)} I_s^* \left. \right] \\
& + i \frac{k_{p-s}}{24} \left( 6I_{3p-s}I_{p-s}I_{3p-s}^* + 6I_{3p-s}I_p e^{ix(k_{3p-s}-k_{3p}-k_{p-s}+k_p)} I_{3p}^* + 6I_{3p-s}I_s e^{ix(k_{3p-s}-k_{2p+s}-k_{p-s}+k_s)} I_{2p+s}^* \right. \\
& + 6I_{3p-s} e^{ix(k_{3p-s}-2k_{p-s}-k_{p+s})} I_{p-s}^* I_{p+s}^* + 3I_{3p-s} e^{ix(k_{3p-s}-k_{p-s}-2k_p)} (I_p^*)^2 \\
& + 6I_{3p-s} e^{ix(k_{3p-s}-k_{p-s}-k_{2p-s}-k_s)} I_{2p-s}^* I_s^* + 6I_{2p}I_{p-s}I_{2p}^* + 6I_{2p}I_{2p-s} e^{ix(k_{2p}-k_{3p}-k_{p-s}+k_{2p-s})} I_{3p}^* \\
& + 6I_{2p}I_p e^{ix(k_{2p}-k_{2p+s}-k_{p-s}+k_p)} I_{2p+s}^* + 6I_{2p} e^{ix(k_{2p}-k_{p-s}-k_p-k_s)} I_p^* I_s^* \\
& + 6I_{2p+s}I_{p-s}I_{2p+s}^* + 6I_{2p+s} e^{ix(k_{2p+s}-k_{p-s}-k_{p+s}-k_s)} I_{p+s}^* I_s^* + 6I_{3p}I_{p-s}I_{3p}^* \\
& + 6I_{3p} e^{ix(-k_{2p}+k_{3p}-k_{p-s}-k_s)} I_{2p}^* I_s^* + 6I_{3p} e^{ix(k_{3p}-k_{p-s}-k_p-k_{p+s})} I_p^* I_{p+s}^* \\
& + 3I_{p-s}^2 I_{p-s}^* + 6I_{p-s}I_{2p-s}I_{2p-s}^* + 6I_{p-s}I_p I_p^* + 6I_{p-s}I_{p+s}I_{p+s}^* + 6I_{p-s}I_s I_s^* \\
& + 3I_{2p-s}^2 e^{ix(-k_{3p-s}-k_{p-s}+2k_{2p-s})} I_{3p-s}^* + 6I_{2p-s}I_p e^{ix(-k_{2p}-k_{p-s}+k_{2p-s}+k_p)} I_{2p}^* \\
& + 6I_{2p-s}I_{p+s} e^{ix(-k_{2p+s}-k_{p-s}+k_{2p-s}+k_{p+s})} I_{2p+s}^* + 6I_{2p-s}I_s e^{ix(-k_{p-s}+k_{2p-s}-k_{p+s}+k_s)} I_{p+s}^* \\
& + 6I_{2p-s} e^{ix(-2k_{p-s}+k_{2p-s}-k_s)} I_{p-s}^* I_s^* + 3I_p^2 e^{ix(-k_{p-s}+2k_p-k_{p+s})} I_{p+s}^* \\
& \left. + 3I_{p+s} e^{ix(-k_{p-s}+k_{p+s}-2k_s)} (I_s^*)^2 \right) \tag{S19}
\end{aligned}$$

$$\begin{aligned}
\frac{dI_s}{dx} = & i \frac{k_s}{8} \left[ 2iI_{2p}\epsilon k_s e^{ix(k_{2p}-k_{2p-s}-k_s)} I_{2p-s}^* + 2iI_{2p+s}\epsilon k_s e^{ix(-k_{2p}+k_{2p+s}-k_s)} I_{2p}^* + 2iI_{3p}\epsilon k_s e^{ix(-k_{3p-s}+k_{3p}-k_s)} I_{3p-s}^* \right. \\
& \left. + 2iI_p\epsilon k_s e^{ix(-k_{p-s}+k_p-k_s)} I_{p-s}^* + 2iI_{p+s}\epsilon k_s e^{ix(-k_p+k_{p+s}-k_s)} I_p^* \right] \\
& + i \frac{k_s}{24} \left( 6I_{3p-s}I_s I_{3p-s}^* + 6I_{3p-s} e^{ix(k_{3p-s}-k_{p-s}-k_{2p-s}-k_s)} I_{p-s}^* I_{2p-s}^* + 6I_{2p}I_p e^{ix(-k_{3p-s}+k_{2p}+k_p-k_s)} I_{3p-s}^* \right. \\
& + 6I_{2p}I_{p+s} e^{ix(k_{2p}-k_{3p}+k_{p+s}-k_s)} I_{3p}^* + 6I_{2p}I_s I_{2p}^* + 6I_{2p} e^{ix(k_{2p}-k_{p-s}-k_p-k_s)} I_{p-s}^* I_p^* \\
& + 6I_{2p+s}I_{p-s} e^{ix(-k_{3p-s}+k_{2p+s}+k_{p-s}-k_s)} I_{3p-s}^* + 6I_{2p+s}I_p e^{ix(k_{2p+s}-k_{3p}+k_p-k_s)} I_{3p}^* + 6I_{2p+s}I_s I_{2p+s}^* \\
& + 6I_{2p+s} e^{ix(k_{2p+s}-k_{2p-s}-2k_s)} I_{2p-s}^* I_s^* + 3I_{2p+s} e^{ix(k_{2p+s}-2k_p-k_s)} I_p^{*2} + 6I_{2p+s} e^{ix(k_{2p+s}-k_{p-s}-k_{p+s}-k_s)} I_{p-s}^* I_{p+s}^* \\
& + 6I_{3p}I_s I_{3p}^* + 6I_{3p} e^{ix(-k_{2p}+k_{3p}-k_{p-s}-k_s)} I_{2p}^* I_{p-s}^* + 6I_{3p} e^{ix(k_{3p}-k_{2p-s}-k_p-k_s)} I_{2p-s}^* I_p^* \\
& + 6I_{p-s}I_{p+s} e^{ix(k_{p-s}-k_{2p-s}+k_{p+s}-k_s)} I_{2p-s}^* + 6I_{p-s}I_s I_{p-s}^* + 6I_{2p-s}I_{p+s} e^{ix(-k_{3p-s}+k_{2p-s}+k_{p+s}-k_s)} I_{3p-s}^* \\
& + 6I_{2p-s}I_s I_{2p-s}^* + 3I_{2p-s} e^{ix(-2k_{p-s}+k_{2p-s}-k_s)} I_{p-s}^{*2} + 3I_p^2 e^{ix(-k_{2p-s}+2k_p-k_s)} I_{2p-s}^* \\
& + 6I_pI_{p+s} e^{ix(-k_{2p}+k_p+k_{p+s}-k_s)} I_{2p}^* + 6I_pI_s I_p^* + 3I_{p+s}^2 e^{ix(-k_{2p+s}+2k_{p+s}-k_s)} I_{2p+s}^* \\
& \left. + 6I_{p+s}I_s I_{p+s}^* + 6I_{p+s} e^{ix(-k_{p-s}+k_{p+s}-2k_s)} I_{p-s}^* I_s^* + 3I_s^2 I_s^* \right) \tag{S20}
\end{aligned}$$

To solve this system we tested different methods in `solve_ivp` function of SciPy library in Python<sup>10</sup>: Explicit Runge-Kutta method of order 5(4), 3(2), 8<sup>11-13</sup>; and implicit multi-step variable-order (1 to 5) method based on a backward differentiation formula for the derivative approximation (BDF)<sup>14</sup>. We ensured that all orders of the Runge-Kutta method give the same solution, which is close to BDF method solution. It is essential to fix the minimal step during the simulation, which is the length of the Unit Cell  $dx = 5dz = 25\mu\text{m}$ , considering smaller steps have no physical meaning. Note that Runge-Kutta methods in `solve_ivp` use adaptive simulation steps, and it could choose simulation steps smaller than the length of a segment of the waveguide corresponding to a single JJ, which leads to divergent solutions. To fix this, we set the relative and the absolute tolerance to large numbers  $\text{rtol} = 1\text{e}+90$ ,  $\text{atol} = 1\text{e}+90$ , and set  $\text{max\_step} = \text{first\_step} = 25\mu\text{m}$ . For the BDF method, we set  $\text{rtol} = 1\text{e}-6$  and  $\text{atol} = 1\text{e}-9$ . The solution of this system by the Explicit Runge-Kutta method of order 3(2) is depicted in Fig. 3. The simulation code used is available online.<sup>15</sup>

## S5. THE DOMINANT PROCESSES BEHIND THG MEDIATED GAIN WITHIN CMT

A simplified version of coupled-mode theory was derived by retaining only the terms essential for capturing the connection between third harmonic strength and signal gain.

$$I'_p = i \frac{k_p \xi}{24} \left( I_p \left( 3 |I_p|^2 + 6 |I_{3p}|^2 \right) \right), \quad I'_{3p} = i \frac{k_{3p} \xi}{24} \left( I_{3p} \left( 6 |I_p|^2 + 3 |I_{3p}|^2 \right) \right) \quad (\text{S21})$$

$$I'_s = i \frac{k_s \epsilon}{8} \left( 2 I_p I_{p-s}^* e^{i(k_p - k_{p-s} - k_s)x} + 2 I_{p+s} I_p^* e^{i(k_{p+s} - k_p - k_s)x} \right) + i \frac{k_s \xi}{24} \left( I_s \left( 6 |I_p|^2 + 6 |I_{3p}|^2 \right) \right) \quad (\text{S22})$$

$$I'_{p-s} = i \frac{k_{p-s} \epsilon}{8} \left( 2 I_p I_s^* e^{i(k_p - k_s - k_{p-s})x} \right) + i \frac{k_{p-s} \xi}{24} \left( I_{p-s} \left( 6 |I_p|^2 + 6 |I_{3p}|^2 \right) \right) \quad (\text{S23})$$

$$I'_{p+s} = i \frac{k_{p+s} \epsilon}{8} \left( 2 I_s I_p e^{i(k_s + k_p - k_{p+s})x} + 2 I_{3p} I_{2p-s}^* e^{i(k_{3p} - k_{2p-s} - k_{p+s})x} \right) + i \frac{k_{p+s} \xi}{24} \left( I_{p+s} \left( 6 |I_p|^2 + 6 |I_{3p}|^2 \right) \right) \quad (\text{S24})$$

$$I'_{2p-s} = i \frac{k_{2p-s} \epsilon}{8} \left( 2 I_{3p} I_{p+s}^* e^{i(k_{3p} - k_{p+s} - k_{2p-s})x} \right) + i \frac{k_{2p-s} \xi}{24} \left( I_{2p-s} \left( 6 |I_p|^2 + 6 |I_{3p}|^2 \right) \right) \quad (\text{S25})$$

Utilizing undepleted pump and third harmonic approximation, Eqs. (S21) yields

$$I_p = I_p(0) \exp \left( i \frac{k_p \xi}{24} \left( 3 |I_p(0)|^2 + 6 |I_{3p}(0)|^2 \right) x \right), \quad I_{3p} = I_{3p}(0) \exp \left( i \frac{k_{3p} \xi}{24} \left( 6 |I_p(0)|^2 + 3 |I_{3p}(0)|^2 \right) x \right) \quad (\text{S26})$$

Making use of the following substitutions

$$Y_s = I_s \exp \left( -i \frac{k_s \xi}{24} \left( 6 |I_p(0)|^2 + 6 |I_{3p}(0)|^2 \right) x \right) \exp \left( i \frac{1}{2} \frac{k_p \xi}{24} 3 |I_p(0)|^2 x \right) \quad (\text{S27})$$

$$Y_{p-s} = I_{p-s}^* \exp \left( i \frac{k_{p-s} \xi}{24} \left( 6 |I_p(0)|^2 + 6 |I_{3p}(0)|^2 \right) x \right) \exp \left( -i \frac{1}{2} \frac{k_p \xi}{24} 3 |I_p(0)|^2 x \right) \quad (\text{S28})$$

$$Y_{p+s} = I_{p+s} \exp \left( -i \frac{k_{p+s} \xi}{24} \left( 6 |I_p(0)|^2 + 6 |I_{3p}(0)|^2 \right) x \right) \exp \left( i \frac{3}{2} \frac{k_p \xi}{24} 3 |I_p(0)|^2 x \right) \quad (\text{S29})$$

$$Y_{2p-s} = I_{2p-s}^* \exp \left( i \frac{k_{2p-s} \xi}{24} \left( 6 |I_p(0)|^2 + 6 |I_{3p}(0)|^2 \right) x \right) \exp \left( i \left( \frac{3}{2} \frac{k_p \xi}{24} 3 |I_p(0)|^2 - \left( \theta + \frac{k_{3p} \xi}{24} 3 |I_{3p}(0)|^2 \right) \right) x \right) \quad (\text{S30})$$

the system Eqs. (S21-S25) can be expressed in a matrix form as presented in the main text.

<sup>1</sup>E. Rizvanov, S. Kern, P. Neilinger, and M. Grajcar, *Journal of Applied Physics* **136**, 174401 (2024).

<sup>2</sup>D. M. Pozar, *Microwave engineering; 3rd ed.* (Wiley, Hoboken, NJ, 2005).

<sup>3</sup>S. Chaudhuri, J. Gao, and K. Irwin, *IEEE Transactions on Applied Superconductivity* **25** (2014).

<sup>4</sup>T. Dixon, J. Dunstan, G. Long, J. Williams, P. Meeson, and C. Shelly, *Phys. Rev. Appl.* **14**, 034058 (2020).

<sup>5</sup>T. Dixon, *Resolving Many Mode Processes in Josephson Travelling Wave Parametric Amplifiers*, Ph.D. thesis, Royal Holloway, University of London (2022).

<sup>6</sup>S. Kern, P. Neilinger, E. Il'ichev, A. Sultanov, M. Schmelz, S. Linzen, J. Kunert, G. Oelsner, R. Stolz, A. Danilov, S. Mahashabde, A. Jayaraman, V. Antonov, S. Kubatkin, and M. Grajcar, *Phys. Rev. B* **107**, 174520 (2023).

<sup>7</sup>M. Malnou, B. T. Miller, J. A. Estrada, K. Genter, K. Cicak, J. D. Teufel, J. Aumentado, and F. Lecocq, "A traveling-wave parametric amplifier and converter," (2024), arXiv:2406.19476 [quant-ph].

<sup>8</sup>L. Planat, A. Ranadive, R. Dassonneville, J. Puertas Martínez, S. Léger, C. Naud, O. Buisson, W. Hasch-Guichard, D. M. Basko, and N. Roch, *Phys. Rev. X* **10**, 021021 (2020).

<sup>9</sup>G. L. Gal, G. Butseraen, A. Ranadive, G. Cappelli, B. Fazlizi, E. Bonet, E. Eyraud, L. Planat, and N. Roch, "Gain compression in josephson traveling-wave parametric amplifiers," (2025), arXiv:2502.03022 [quant-ph].

<sup>10</sup>"Scipy documentation,".

<sup>11</sup>P. Bogacki and L. Shampine, *Applied Mathematics Letters* **2**, 321 (1989).

<sup>12</sup>J. Dormand and P. Prince, *Journal of Computational and Applied Mathematics* **6**, 19 (1980).

<sup>13</sup>E. Hairer, S. Norsett, and G. Wanner, *Solving Ordinary Differential Equations I: Nonstiff Problems*, Vol. 8 (1993).

<sup>14</sup>L. F. Shampine and M. W. Reichelt, *SIAM Journal on Scientific Computing* **18**, 1 (1997).

<sup>15</sup>E. Rizvanov, "Coupled mode theory simulator for ptwpa," <https://github.com/EmilRizvanov/CMT3> (2025), gitHub repository.
